# Supplementary material for: Pathways from nucleation to raindrops
Source: arXiv:2410.11072 source file (2024-10-14)
Supplement: Supplementary file 1 [file SupMatCollisionPRF.pdf]

# Pathways from nucleation to raindrops. Supplementary Material

F. Poydenot, B. Andreotti

*Laboratoire de Physique de l'Ecole Normale Supérieure (LPENS), CNRS UMR 8023,  
Ecole Normale Supérieure, Université PSL, Sorbonne Université, and Université de Paris, 75005 Paris,  
France*

(Dated: 11 October 2024)

The Supplementary Material describes the detailed set of equations for the kernel, the numerical integration scheme of the Smoluchowski equation and a validation of the numerical scheme by an analytic solution.

## I. HYDRODYNAMICS

### A. Terminal velocity

We consider a drop of mass  $m$ , density  $\rho_\ell$  and radius  $R$ . The mass of one water molecule is denoted  $m_1$ . It is associated with a radius  $\mathcal{A}$  defined such that this mass is uniformly distributed over a sphere of radius  $\mathcal{A}$  at the density  $\rho_\ell$ :  $m_1 = 4\pi\rho_\ell\mathcal{A}^3/3$ . There are two inertial subregimes, controlled by the droplet Reynolds number  $\mathcal{R} = \rho_g Va/\eta_g$ . A drop between  $10\ \mu\text{m}$  and  $500\ \mu\text{m}$  ( $10^{-2} < \mathcal{R} < 10^2$ ) remains spherical, but the flow around it cannot be described accurately by a viscous flow. Drops above  $500\ \mu\text{m}$  slightly deform into an oblate spheroid; drops above  $1000\ \mu\text{m}$  undergo large deformations and oscillate. In these cases, the drag coefficient does not depend solely on  $\mathcal{R}$  anymore, but also on surface tension. We neglect drop oscillations, but we take into account the deformation of the largest drops. Large drops are pancake-shaped, with a thickness independant of their size that scales as the capillary length  $\ell_\gamma = \sqrt{\gamma/\rho_\ell g}$ , and fall at a speed independant of their size. Balance between hydrodynamic stress and surface tension yields<sup>1,2</sup>

$$U^t = \left( \frac{8}{3C_\gamma} \frac{(\gamma\rho_\ell g)^{1/2}}{\rho_g} \right)^{1/2}, \quad (1)$$

with  $C_\gamma = 0.92$  from the data of Reyssat *et al.*<sup>1</sup> Flow in the inertial regime can be described using the drag coefficient  $C_d$  such that

$$\frac{d}{dt} \vec{V}(t) = \frac{3}{8} C_d \frac{\rho_g}{\rho_\ell} \frac{V \vec{V}(t)}{a} + \vec{g}, \quad (2)$$

The flattening of the drop when  $a$  approaches the capillary length leads to an effective surface larger than  $\pi a^2$ , if  $a$  remains a pseudo-radius determined from the drop mass. The height tends to a constant  $\sim \ell_\gamma$  for large drops, obeying the phenomenological relation  $\sim \left(1 + C_\gamma \left(\frac{a}{\ell_\gamma}\right)^3\right)^{-1/3} a$ . Introducing the surface correction, the drag coefficient  $C_d$  can be phenomenologically be written as:

$$C_d = \left( C_\infty^{1/2} \left(1 + C_\gamma \left(\frac{a}{\ell_\gamma}\right)^3\right)^{1/6} + \left(\frac{12\nu}{Va}\right)^{1/2} \right)^2, \quad (3)$$

with  $C_\infty$  a phenomenological calibrated constant ( $C_\infty = 0.26$  and  $C_\gamma = 0.1$  from fitting data by Gunn and Kinzer<sup>3</sup>). The terminal velocity  $U^t$  reads:

$$C_\infty^{1/2} \left(1 + C_\gamma \left(\frac{a}{\ell_\gamma}\right)^3\right)^{1/6} U^t + \left(\frac{12\nu}{a}\right)^{1/2} (U^t)^{1/2} = \left(\frac{8}{3} \frac{\rho_\ell}{\rho_g} ga\right)^{1/2} \quad (4)$$

We make  $U^t$  dimensionless using the terminal velocity of drop of radius  $\mathcal{A}$ , computed as if it was in the turbulent drag regime. Introducing the dimensionless droplet mass  $\tilde{x} = m/m_1$ , we get:

$$U^t = \nu \tilde{U} = \left( \frac{8\rho_\ell g \mathcal{A}}{3\rho_g C_\infty} \right)^{1/2} \tilde{U}(\tilde{x}) \quad (5)$$

The velocity  $\mathcal{V}$  is equal to 4 mm/s.  $\tilde{U}(\tilde{x})$  is defined by

$$\left(1 + \frac{\tilde{x}}{i_\gamma}\right)^{1/6} \tilde{U} + \frac{i_\nu^{1/4}}{\tilde{x}^{1/6}} \tilde{U}^{1/2} = \tilde{x}^{1/6} \quad (6)$$

with

$$i_\nu = \left(\frac{54\rho_g\nu^2}{C_\infty\rho_\ell g\mathcal{A}^3}\right) \simeq 8.1 \cdot 10^{17}, \quad i_\gamma = \frac{\ell_\gamma^3}{C_\gamma\mathcal{A}^3} \simeq 2.8 \cdot 10^{22} \quad (7)$$

$\tilde{U}$  presents three successive scaling regimes: for  $\tilde{x} \ll \tilde{x}_\nu$ ,  $\tilde{U} \propto \tilde{x}^{2/3}$ , for  $\tilde{x}_\nu \ll \tilde{x} \ll \tilde{x}_\gamma$ ,  $\tilde{U} \propto \tilde{x}^{1/6}$  and for  $\tilde{x} \gg \tilde{x}_\gamma$ ,  $\tilde{U} \propto i_\gamma^{1/6}$ .

## B. Collision kernel

As described in details in the companion paper,<sup>4</sup> the kernel is written under the form:

$$K = \pi(R_1 + R_2)^2 E_d q(\text{Pe}) |U_1^t - U_2^t|, \quad \text{with} \quad \text{Pe} = \frac{|U_1^t - U_2^t|(R_1 + R_2)}{D_1 + D_2}, \quad D_i = \frac{k_B T}{6\pi\eta_g R_i}. \quad (8)$$

In the code, the product  $E_d q(\text{Pe})$  is decomposed as

$$E_d q(\text{Pe}) = \frac{4}{\text{Pe}} + E + \text{corrective terms}(\text{Pe}, R_1, R_2), \quad (9)$$

with  $E$  the usual efficiency computed using deterministic (not Monte-Carlo) equations and the corrective terms, depending on the mechanisms investigated, computed using the difference between deterministic computations and Monte-Carlo simulations.  $4/\text{Pe}$  is the pure diffusion asymptotic limit. Efficiencies for the binary drop calculations of the companion paper are fitted on a limited set of analytic functions (18 in total for all mechanisms) such that computation of the kernels is both fast, accurate and asymptotically correct, both in the low-Péclet (pure diffusion) and high-Stokes (geometric gravity collisions with  $E = 1$ ) limits.

## II. NUMERICAL SCHEME

### A. Dimensionless equations

Denoting by  $n(m, t)$  the density of drops of mass  $m$ , the Smoluchowski equation reads:<sup>5</sup>

$$\frac{\partial n}{\partial t} = \frac{1}{2} \int_0^m dx n(m-x)n(x)K(m-x, x) - n(m) \int_0^\infty dx n(x)K(m, x) \quad (10)$$

We make the equation dimensionless using the mass scale  $m_1$ . Masses  $x$  become  $\tilde{x} = x/m_1$ . The diffuso-gravitational kernel is

$$K(x, y) = K_0 E_d(\tilde{x}, \tilde{y}) q(\text{Pe}) \left(\tilde{x}^{1/3} + \tilde{y}^{1/3}\right)^2 \left|\tilde{U}(\tilde{x}) - \tilde{U}(\tilde{y})\right| = K_0 \tilde{K}(\tilde{x}, \tilde{y}) \quad \text{with} \quad K_0 = \pi \mathcal{A}^2 \mathcal{V} \quad (11)$$

Using  $\psi$  as the number scale such that  $n = \psi m_1^{-1} \tilde{n}$  and  $T$  the time scale, we get

$$\frac{\partial \tilde{n}}{\partial \tilde{t}} = \psi T K_0 \left( \frac{1}{2} \int_0^{\tilde{x}} d\tilde{y} \tilde{n}(\tilde{x} - \tilde{y}) \tilde{n}(\tilde{x}) \tilde{K}(\tilde{x} - \tilde{y}, \tilde{y}) - \tilde{n}(\tilde{x}) \int_0^\infty d\tilde{y} \tilde{n}(\tilde{y}) \tilde{K}(\tilde{x}, \tilde{y}) \right) \quad (12)$$

$$(13)$$

This sets the typical time scale  $T$

$$T = K_0^{-1} \psi^{-1} = \frac{1}{\pi \psi \mathcal{A}^2 \mathcal{V}} \quad (14)$$

In the code, masses are adimensionalized by an arbitrary scale  $M = \gamma m_1$ .  $n$  becomes  $n = \psi M^{-1} \tilde{n}$ , the kernel becomes  $K(x, y) = \pi \mathcal{A}^2 \mathcal{V} \gamma^{2/3} \tilde{K}(\tilde{x}, \tilde{y})$ . This shifts the time scale:

$$T = K_0^{-1} \gamma^{-2/3} \psi^{-1} = \frac{1}{\pi \psi \mathcal{A}^2 \mathcal{V} \gamma^{2/3}} \quad (15)$$

In the code,  $\gamma = 38,084,183$  such that bins range from 64 nm to 7.7 mm.

## B. Discrete equations

We consider the following system for  $i = 1 \dots i_{\max}$  and  $n_i$  the number density of  $i$ -sized clusters (i.e. droplets of mass  $m = i m_1$ )

$$\frac{dn_i}{dt} = \frac{1}{2} \sum_{j=1}^i K(i-j, j) n_j n_{i-j} - \sum_j K(i, j) n_i n_j. \quad (16)$$

In the double limit of  $m_1 \rightarrow 0$ ,  $i \rightarrow \infty$ , this infinite set of equations reduces to the integro-differential equation (10) with the same kernel  $K$ , replacing the number density of species  $i$  with the now continuous mass density  $n(m)$ .

## C. Mass discretization

We wish to simulate, in fine, the equation up to the macroscopic scale, say to millimetric drops. This would correspond to a maximum value  $i \sim 10^{23}$  while long integers only go to  $10^{19}$ . We now refer to the bin label with  $i$ , and to the droplet mass (in units of  $m_1$ ) with  $x_i$ . The bin  $i$  goes from  $x_{i-1} + 1$  to  $x_i$ . We define:

$$N_i = \sum_{l=x_{i-1}+1}^{x_i} n_l, \quad (17)$$

the number density summed over the bin  $i$ . The exact equation governing  $N_i$  reads:

$$\frac{dN_i}{dt} = \frac{1}{2} \sum_{l=x_i}^{x_{i+1}-1} \sum_{j=1}^l \tilde{K}(l-j, j) n_j n_{l-j} - \sum_j \tilde{K}(l, j) n_l n_j \quad (18)$$

We consider a series of bins labelled from  $i = 1$  to  $i = L_m = 550$ . From  $i = 1$  to  $i = L = 17$ , we use a simple constant binning. Bin  $i \leq L$  contains the rescaled mass  $m/\gamma m_1 = i$ . Above, we introduce a logarithmic dependence of  $x_i$  with  $i$ , such that the lin and log zone match in  $i = L - 1$  and  $i = L$ . By convention, we add  $x_0 = 0$ . From  $i = L$  to  $i = R = 111$ , we define

$$x_i = \text{Int} \left( L \exp \left[ \ln \left( \frac{L}{L-1} \right) (i - L) \right] \right) \quad (19)$$

For  $i > R$ , we store the masses with real numbers:

$$x_i = L \exp \left[ \ln \left( \frac{L}{L-1} \right) (i - L) \right] \quad (20)$$

and use the approximate sums:

$$\sum_{l=x_{i-1}+1}^{x_i} f(l) \simeq \int_{l=x_{i-1}+1/2}^{x_i+1/2} f(l) dl \quad (21)$$

$$\simeq \delta_i \sum_{l=1}^{x_{R+1}-x_R} f(x_{i-1} + 1/2 + (l - 1/2) \delta_i), \quad (22)$$

replacing the subintervals of size 1 by a subinterval of size

$$\delta_i = \frac{x_i - x_{i-1}}{x_R - x_{R-1}} > 1. \quad (23)$$

At the second order, we compute the quadratic interpolation between  $i - 1$ ,  $i$  and  $i + 1$  to determine the upwind biased estimate of the flux between  $i$  and  $i + 1$ :

$$n_l = a_i + (b_i - a_i)(l - x_i) + c_i(l - x_i)(l - x_i - 1) \quad (24)$$

The parametrisation is chosen such that  $a_i$  is the estimate of  $n_{x_i}$  and  $b_i$  the estimate of  $n_{x_i + 1}$ . We solve for  $a_i$ ,  $b_i$  and  $c_i$  obeying:

$$N_{i+1} = \sum_{l=x_i+1}^{x_{i+1}} n_l = \sum_{l=x_i+1}^{x_{i+1}} [a_i + (b_i - a_i)(l - x_i) + c_i(l - x_i)(l - x_i - 1)] \quad (25)$$

$$N_i = \sum_{l=x_{i-1}+1}^{x_i} n_l = \sum_{l=x_{i-1}+1}^{x_i} [a_i + (b_i - a_i)(l - x_i) + c_i(l - x_i)(l - x_i - 1)] \quad (26)$$

$$N_{i-1} = \sum_{l=x_{i-2}+1}^{x_{i-1}} n_l = \sum_{l=x_{i-2}+1}^{x_{i-1}} [a_i + (b_i - a_i)(l - x_i) + c_i(l - x_i)(l - x_i - 1)] \quad (27)$$

$$(28)$$

For  $i < L$ , we simply recover:  $a_i = N_i$ ,  $b_i = N_{i+1}$  and  $c_i = N_i - (N_{i+1} + N_{i-1})/2$ . The integration scheme is first order in time, with the single step:

$$\delta N_i = \left( \frac{1}{2} \sum_{l=x_i}^{x_{i+1}-1} \sum_{j=1}^l \tilde{K}(l-j, j) n_j n_{l-j} - \sum_j \tilde{K}(l, j) n_l n_j \right) \delta t \quad (29)$$

which is an equation always leading to the growth of droplets. For the boundary condition, we impose  $N_I = 0$ .

#### D. Interpolation for the collision term

Regarding the collision, we scan all pairs of bins  $i < j$ , which should lead to a transfer of mass from bins ranging from  $x_{i-1} + 1$  to  $x_i$  and  $x_{j-1} + 1$  to  $x_j$  to the sum, which goes from  $x_{i-1} + x_{j-1} + 2$  to  $x_i + x_j$ . The result is spread over bins  $k - 1$  and  $k$ . We can compute explicitly the decomposition:

$$\tilde{K}(l, m) n_l n_m \quad (30)$$

and resum over  $l$  and  $m$ . At the lowest order, we consider that  $n_i$  is uniform between  $x_{i-1} + 1$  and  $x_i$ . Then, we compute the weight in advance to split the result between the bins  $k(i, j) - 1$  and  $k(i, j)$ . Altogether, we present the result under the transform:  $(i, j) \rightarrow k(i, j) + l$  at a rate  $s_{i,j,l} N_i N_j$ , where  $s_{i,j,l}$  is the collision stencil, which depends only on the binning such that

$$n_l n_m = (a_i + (b_i - a_i)(l - x_i) + c_i(l - x_i)(l - x_i - 1)) (a_j + (b_j - a_j)(m - x_j) + c_j(m - x_j)(m - x_j - 1)). \quad (31)$$

The stencil is computed once, then stored.

#### E. Distributions used

The initial condition for all computations in the main text is the lognormal distribution

$$n_l(m) = \frac{\psi}{\sqrt{2\pi}\sigma_{LN}m} \exp \left[ -\frac{(\ln(m) - \mu)^2}{2\sigma_{LN}^2} \right] \quad (32)$$

with  $\sigma_{LN} = 0.4$  [outside of Fig. 5(b), where it varies from 0.1 to 1.5] and  $\mu$  corresponding to the mass of a droplet of  $R = 4 \mu\text{m}$ .  $R_\infty$  is the radius corresponding to the initial mean mass  $\int mn(m)dm / \int n(m)dm$ . In practice, we vary  $\mu$  and recompute  $R_\infty$  from the initial distribution in the numerical data.

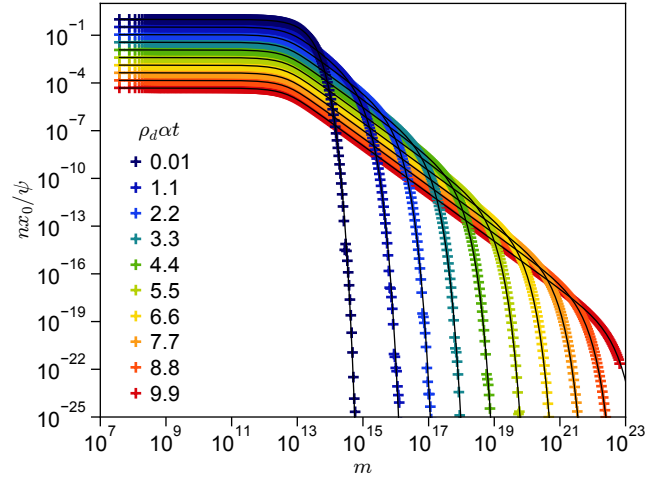

FIG. 1. Validation of the numerical scheme by the exact Golovin<sup>6</sup> solution. Colored crosses: numerical solution at different dimensionless times  $\rho_d \alpha t$ . Solid black lines: analytic solution given by Eq. (34).

### III. VALIDATION OF THE NUMERICAL SCHEME

Golovin<sup>6</sup> (see also Berry<sup>7</sup>) showed that for the kernel  $K = \alpha(x + y)$  and the initial condition

$$n_0(x) = \psi/x_0 \exp(-x/x_0), \quad (33)$$

with  $x_0 = \rho_d/\psi$  the initial droplet mass,  $\psi$  the initial droplet concentration and  $\rho_d$  the liquid water content. The exact solution to the problem is

$$n(x, t) = \psi x^{-1} \tau^{-1/2} (1 - \tau) I_1(2\tau^{1/2}s) \exp[-(1 + \tau)s], \quad \tau = 1 - \exp(-L\alpha t), \quad s = x/x_0, \quad (34)$$

with  $I_1$  the modified Bessel function of the first kind. Figure 1 shows the numerical and analytic solutions. Agreement between the two is excellent for the whole range of sizes, and very slightly degrades at the very far end of the tails where the size distribution becomes vanishingly small, much below the values used to support the calculations in the main text.

<sup>1</sup>É. Reyssat, F. Chevy, A.-L. Biance, L. Petitjean, and D. Quéré, “Shape and instability of free-falling liquid globules,” *Europhysics Letters* (EPL) **80**, 34005 (2007).

<sup>2</sup>H. Pruppacher and J. Klett, *Microphysics of Clouds and Precipitation* (Springer Netherlands, Dordrecht, 2010).

<sup>3</sup>R. Gunn and G. D. Kinzer, “The terminal velocity of fall for water droplets in stagnant air,” *Journal of Meteorology* **6**, 243–248 (1949).

<sup>4</sup>F. Poydenot and B. Andreotti, “Gap in drop collision rate between diffusive and inertial regimes explains the stability of fogs and non-precipitating clouds,” *Journal of Fluid Mechanics* **987**, A37 (2024).

<sup>5</sup>M. von Smoluchowski, “Three Presentations on Diffusion, Molecular Movement According to Brown and Coagulation of Colloid Particles,” *Physikalische Zeitschrift* **17**, 557–571 (1916).

<sup>6</sup>A. M. Golovin, “The solution of the coagulation equation for cloud droplets in a rising air current,” *Izv. Geophys. Ser* **5**, 82–4 (1963).

<sup>7</sup>E. X. Berry, “Cloud droplet growth by collection,” *Journal of the Atmospheric Sciences* **24**, 688–701 (1967).
